# Supplementary material for: Fast, Cheap, and Fair? Evaluating Decision Models
Source: arXiv:2611.04510 source file (2026-11-03)
Supplement: Supplementary file 1 [file discrim_eval.tex]

% \begin{lstlisting}[style=prompt,title={Decision models: state (one yes/no question; $p(\text{yes})$ is the model's probability)}]
% <filled_template>

% Please answer the above question with either "yes" or "no".
% \end{lstlisting}

% \begin{lstlisting}[style=prompt,title={Generative models: user prompt (no system instruction; output \{"p\_yes": number\})}]
% <filled_template>

% Please answer the above question with either "yes" or "no".

% Give the probability (0 to 1) that your answer is "yes".
% \end{lstlisting}

% discrim-eval prompts, set as one full-width float.
% Uses the listings package.
\lstdefinestyle{promptde}{
  basicstyle=\ttfamily\fontsize{6.5}{7.6}\selectfont,
  breaklines=true,
  breakatwhitespace=true,
  columns=fullflexible,
  frame=single,
  framesep=3pt,
  aboveskip=2pt,
  belowskip=2pt,
  float=false
}
\begin{figure}[t]
\centering
\begin{minipage}[t]{0.485\textwidth}
\begin{lstlisting}[style=promptde,title={Decision models: state}]
<filled_template>

Please answer the above question with either "yes" or "no".
\end{lstlisting}
\end{minipage}\hfill
\begin{minipage}[t]{0.485\textwidth}
\begin{lstlisting}[style=promptde,title={Generative models: user prompt}]
<filled_template>

Please answer the above question with either "yes" or "no".

Give the probability (0 to 1) that your answer is "yes".
\end{lstlisting}
\end{minipage}
\caption{Prompts for \dsdiscrim{}. \texttt{<filled\_template>} is the
scenario text of \citet{tamkin2023evaluating}. \dms{} answer one yes/no question and return $\pyes$ directly; \gms{} receive no system instruction and return \texttt{\{"p\_yes": number\}}.}
\label{fig:app-prompt-de}
\end{figure}
