# Supplementary material for: Fast, Cheap, and Fair? Evaluating Decision Models
Source: arXiv:2611.04510 source file (2026-11-03)
Supplement: Supplementary file 2 [file discrim_eval.tex]

\begin{table}[t]
\centering
\footnotesize
\setlength{\tabcolsep}{3pt}
\begin{tabular}{lp{4.6cm}}
\toprule
Attribute & Values \\
\midrule
Age    & 20--100 in steps of 10 (ref.\ 60) \\
Gender & Male (ref.), female, non-binary \\
Race   & White (ref.), Black, Asian, Hispanic, Native American \\
\midrule
Scenarios & 70 decisions (e.g.\ loans, housing, hiring) \\
Profiles  & 135 per scenario ($9 \times 3 \times 5$) \\
Variants  & Explicit (attributes stated); implicit (race and gender via name and pronouns) \\
Prompts   & 9{,}450 per variant, 18{,}900 in total \\
\bottomrule
\end{tabular}
\caption{Demographic attributes and size of \dsdiscrim dataset.}
\label{tab:app-de}
\end{table}
